# Supplementary material for: Unsupervised Dense Information Retrieval with Contrastive Learning
Source: arXiv:2112.09118 source file (2022-08-29)
Supplement: Supplementary file 1 [file appendix.tex]

\newpage

\appendix
\section{Additional experimental results}

\begin{table*}[t]
    \tiny
    \setlength{\tabcolsep}{.5em}
    \resizebox{\textwidth}{!}{
    \begin{tabular}{@{}l  c  c  c c c c c  c c  c@{}}
        \toprule
        \multicolumn{1}{@{}l}{\textbf{Model ($\rightarrow$)}} &
        \multicolumn{1}{c}{Lexical}   &
        \multicolumn{1}{c}{Sparse}   &
        \multicolumn{5}{c}{Dense / Neural} &
        \multicolumn{2}{c}{Reranking} &
        \multicolumn{1}{c@{}}{Ours} \\ 
        \cmidrule(r){1-1}
        \cmidrule(lr){2-2}
        \cmidrule(lr){3-3}
        \cmidrule(lr){4-8}
        \cmidrule(lr){9-10}
        \cmidrule(lr){11-12}
        \multicolumn{1}{@{}l}{\textbf{Dataset ($\downarrow$)}} &
        \multicolumn{1}{c}{\textbf{BM25}} &
        \multicolumn{1}{c}{\textbf{SPARTA}} &
        \multicolumn{1}{c}{\textbf{USE-QA}} &
        \multicolumn{1}{c}{\textbf{DPR}} &
        \multicolumn{1}{c}{\textbf{ANCE}} &
        \multicolumn{1}{c}{\textbf{SBERT}} &
        \multicolumn{1}{c}{\textbf{GenQ}} &
        \multicolumn{1}{c}{\textbf{BM25+CE}} &
        \multicolumn{1}{c}{\textbf{ColBERT}} &
        \multicolumn{1}{c@{}}{\textbf{M+B}} \\
        \midrule
  MSMARCO & 21.8 & 35.1$^\ddagger$ & 25.9 & 17.7 & 38.8$^\ddagger$ & \underline{38.9}$^\ddagger$ & \underline{38.9}$^\ddagger$ & 38.4$^\ddagger$ & \textbf{42.5}$^\ddagger$ & 35.6$^\ddagger$\\  \midrule 
   TREC-COVID    & 61.6 & 53.8 & 52.8 & 33.2 & 65.4 & 48.2 & 55.4 & \underline{66.7} & \textbf{67.7} & 43.8 \\
   BioASQ        & \textbf{51.4} & 35.1 & 09.3 & 12.7 & 30.6 & 29.5 & 35.1 & \underline{48.9} & 47.4 & - \\
   NFCorpus      & 29.7 & 30.1 & 25.2 & 18.9 & 23.7 & 25.7 & 29.3 & 30.3 & \underline{30.5} & \bf 32.4\\ \midrule
   NQ            & 31.0 & 39.8 & 18.0 & 47.4$^\ddagger$ & 44.6 & 45.0 & 36.0 & \underline{51.6} & \textbf{52.4} &   44.3 \\
   HotpotQA      & 60.1 & 49.2 & 25.8 & 39.1 & 45.6 & 51.3 & 49.7 & \textbf{70.1} & 59.3 & \underline{64.4} \\
   FiQA-2018     & 23.9 & 19.8 & 26.4 & 11.2 & 29.5 & 25.8 & 28.4 & \textbf{32.6} & \underline{31.7} & 27.7 \\ \midrule
   Signal-1M (RT)& \textbf{38.8} & 25.2 & 24.1 & 15.5 & 24.9 & 26.1 & 25.7 & \underline{30.8} & 27.4 & - \\ \midrule
   TREC-NEWS     & 37.1 & 25.8 & 34.0 & 16.1 & 38.2 & 36.7 & 36.9 & \textbf{43.0} & \underline{39.3} & - \\ \midrule
   ArguAna       & \underline{44.1} & 27.9 & ~4.8 & 17.5 & 41.5 & 42.9 & \textbf{51.7} & 23.3 & - & - \\
   T\'ouche-2020 & \textbf{60.5} & 23.1 & 25.2 & 12.7 & 28.4 & 24.9 & 22.6 & 37.8 & 27.5 & \underline{38.2}\\ \midrule
   CQADupStack   & 31.6 & 25.7 & 23.6 & 15.3 & 29.6 & 30.6 & 33.9 & \underline{34.8} & \textbf{35.0} & - \\
   Quora         & 74.2 & 63.0 & 76.7 & 24.8 & 85.2 & \textbf{85.5} & 85.3 & 77.8 & \underline{85.4} & 84.9 \\ \midrule
   DBPedia       & 28.8 & 31.4 & 23.8 & 26.3 & 28.1 & 33.9 & 32.0 & \underline{38.0} & \textbf{39.2} & \colorbox{green!30}{35.8} \\ \midrule
   SCIDOCS       & \textbf{15.6} & 12.6 & 10.4 & ~7.7 & 12.2 & 13.3 & 14.8 & \underline{15.4} & 14.5 & \underline{15.4} \\ \midrule
   FEVER         & 64.8 & 59.6 & 54.6 & 56.2 & 66.9 & 67.0 & 64.1 & \textbf{79.3} & \underline{77.1} & \colorbox{green!30}{74.5} \\
   Climate-FEVER & 17.9 & ~8.2 & 11.3 & 14.8 & 19.8 & 20.5 & \underline{22.0} & \textbf{24.6} & 18.4 & 19.6 \\
   SciFact       & 62.0 & 58.2 & 31.2 & 31.8 & 50.7 & 53.1 & 59.2 & 52.4 & \underline{67.1} &\textbf{69.1} \\ \midrule
   AVERAGE       & 41.9 & 34.6 & 28.0 & 23.3 & 39.1 & 38.8 & 40.1 & \textbf{44.7} & \underline{43.7} & - \\
        \bottomrule
    \end{tabular}}
    \caption{\textbf{Comparison between universal retrievers.} We report the nDCG@10 and Recall@100 performances on BEIR datasets. 
    For this evaluation, we finetune our pre-trained model on MSMARCO, following \aj{XX cite why it is common practice}.
    The models are applied with no finetuning on each dataset.
    The best performance is in \textbf{bold}, and the second best performance is \underline{underlined}.
    $\ddagger$ indicates the in-domain performances.}
    \label{tab:results}
\end{table*}

\begin{table*}[t!]
    \tiny
    \resizebox{\textwidth}{!}{\begin{tabular}{@{}l  c  c  c c c c c  c c  c c@{}}
        \toprule
        \multicolumn{1}{l}{\textbf{Model ($\rightarrow$)}} &
        \multicolumn{1}{c}{Lexical}   &
        \multicolumn{1}{c}{Sparse}   &
        \multicolumn{5}{c}{Dense / Neural} &
        \multicolumn{2}{c}{Reranking} &
        \multicolumn{2}{c}{Ours} \\ 
        \cmidrule(lr){1-1}
        \cmidrule(lr){2-2}
        \cmidrule(lr){3-3}
        \cmidrule(lr){4-8}
        \cmidrule(lr){9-10}
        \cmidrule(lr){11-12}
        \multicolumn{1}{l}{\textbf{Dataset ($\downarrow$)}} &
        \multicolumn{1}{c}{\textbf{BM25}} &
        \multicolumn{1}{c}{\textbf{SPARTA}} &
        \multicolumn{1}{c}{\textbf{USE-QA}} &
        \multicolumn{1}{c}{\textbf{DPR}} &
        \multicolumn{1}{c}{\textbf{ANCE}} &
        \multicolumn{1}{c}{\textbf{SBERT}} &
        \multicolumn{1}{c}{\textbf{GenQ}} &
        \multicolumn{1}{c}{\textbf{BM25+CE}} &
        \multicolumn{1}{c}{\textbf{ColBERT}} & 
        \multicolumn{1}{c}{\textbf{M+B}} &
        \multicolumn{1}{c}{\textbf{+Ft.}}\\
        \midrule
\multicolumn{12}{c}{Recall@100}\\ 
\midrule
   MSMARCO       & 62.1 & 79.3$^\ddagger$ & 72.0 & 55.2 & \underline{85.2}$^\ddagger$ & 84.7$^\ddagger$ & 84.7$^\ddagger$ & 62.1$^\ddagger$ &  \textbf{86.5}$^\ddagger$ & 60.9 & {87.5} \\
   TREC-COVID    & 44.7$^\star$ & 40.9$^\star$ & 33.9$^\star$ & 21.2$^\star$ & \underline{45.7}$^\star$ & 34.4$^\star$ & 44.2$^\star$ & 44.7$^\star$ & \textbf{46.4}$^\star$ \\
   BioASQ        & \textbf{71.6} & 35.1 & 14.5 & 25.6 & 46.3 & 46.6 & 57.7 & \textbf{71.6} & \underline{64.5} \\
   NFCorpus      & 19.6 & 24.3 & \textbf{27.3} & 20.8 & 23.2 & 23.5 & \underline{27.2} & 19.6 & 25.4 & {28.5} & {29.2} \\
   NQ            & 75.3 & 78.7 & 60.5 & \underline{88.0}$^\ddagger$ & 83.6 & 85.8 & 84.5 & 75.3 & \textbf{91.2} & 67.2 & {91.8} \\
   HotpotQA      & \textbf{75.7} & 65.1 & 39.8 & 59.1 & 57.8 & 63.7 & 62.4 & \textbf{75.7} & \underline{74.8} & 61.0 & {79.1}\\
   FiQA-2018     & 50.5 & 44.6 & 60.1 & 34.2 & 58.1 & 54.0 & \textbf{60.9} & 50.5 & \underline{60.3} & 44.0 & 59.5\\
   Signal-1M (RT)& \textbf{37.6} & 27.0 & 26.6 & 16.2 & 23.9 & 26.3 & 27.1 & \textbf{37.6} & \underline{28.3} \\
   TREC-NEWS     & \textbf{40.1} & 26.2 & 38.1 & 21.5 & \underline{39.8} & 36.7 & 39.5 & \textbf{40.1} & 36.7 \\
   ArguAna       & 93.1 & 89.3 & 45.4 & 75.1 & 93.7 & \underline{94.5} & \textbf{97.9} & 93.1 & 91.4 & 92.8 & 92.7 \\
   T\'ouche-2020 & \textbf{46.3} & 25.7 & 25.7 & 17.1 & 30.7 & 30.0 & 27.3 & \textbf{46.3} & \underline{30.9} & 26.3 & 25.0 \\
   CQADupStack   & 58.8 & 52.1 & 54.6 & 40.3 & 57.9 & 59.6 & \textbf{67.2} & 58.8 & \underline{62.4} \\
   Quora         & 94.8 & 89.6 & 97.8 & 47.0 & \underline{98.7} & \textbf{98.9} & \textbf{98.9} & 94.8 & \textbf{98.9} & 95.9 & {98.9} \\
   DBPedia       & 38.4 & \underline{41.1} & 28.1 & 34.9 & 31.9 & 40.3 & 39.6 & 38.4 & \textbf{46.1} & 37.9 & {51.5} \\
   SCIDOCS       & \textbf{34.6} & 29.7 & 25.5 & 21.9 & 26.9 & 29.6 & 33.4 & \textbf{34.6} & \underline{34.4} & {36.8} & {36.2}\\
   FEVER         & 90.8 & 84.3 & 85.0 & 84.0 & 90.0 & 91.4 & \underline{92.0} & 90.8 & \textbf{93.4} & 92.0 & {94.7} \\
   Climate-FEVER & 38.3 & 22.7 & 34.6 & 39.0 & 44.5 & \underline{44.8} & \textbf{51.7} & 38.3 & 44.4 & 46.3 & 49.2 \\
   SciFact       & 83.8 & 86.3 & 63.1 & 72.7 & 81.6 & 84.9 & \textbf{89.2} & 83.8 & \underline{87.8} & {96.1} & {93.6} \\
   \midrule
   AVERAGE       & 58.7 & 52.3 & 46.3  & 43.0 & 56.6 & 57.2 & \underline{60.3} & 58.7 & \textbf{61.3} \\
   \midrule
   \multicolumn{12}{c}{NDCG@10}\\
   \midrule
   MSMARCO & 21.8 & 35.1$^\ddagger$ & 25.9 & 17.7 & 38.8$^\ddagger$ & \underline{38.9}$^\ddagger$ & \underline{38.9}$^\ddagger$ & 38.4$^\ddagger$ & \textbf{42.5}$^\ddagger$ & 16.8 & 35.6\\
   TREC-COVID    & 61.6 & 53.8 & 52.8 & 33.2 & 65.4 & 48.2 & 55.4 & \underline{66.7} & \textbf{67.7} & 21.4 & 43.8 \\
   BioASQ        & \textbf{51.4} & 35.1 & 09.3 & 12.7 & 30.6 & 29.5 & 35.1 & \underline{48.9} & 47.4 \\
   NFCorpus      & 29.7 & 30.1 & 25.2 & 18.9 & 23.7 & 25.7 & 29.3 & \underline{30.3} & \textbf{30.5} &  29.9 & \colorbox{blue!30}{32.4}\\
   NQ            & 31.0 & 39.8 & 18.0 & 47.4$^\ddagger$ & 44.6 & 45.0 & 36.0 & \underline{51.6} & \textbf{52.4} &  18.4 & 44.3 \\
   HotpotQA      & \underline{60.1} & 49.2 & 25.8 & 39.1 & 45.6 & 51.3 & 49.7 & \textbf{70.1} & 59.3 & 38.4 & \colorbox{green!30}{64.4} \\
   FiQA-2018     & 23.9 & 19.8 & 26.4 & 11.2 & 29.5 & 25.8 & 28.4 & \textbf{32.6} & \underline{31.7} & 16.8 & 27.7\\
   Signal-1M (RT)& \textbf{38.8} & 25.2 & 24.1 & 15.5 & 24.9 & 26.1 & 25.7 & \underline{30.8} & 27.4 \\
   TREC-NEWS     & 37.1 & 25.8 & 34.0 & 16.1 & 38.2 & 36.7 & 36.9 & \textbf{43.0} & \underline{39.3} \\
   ArguAna       & \underline{44.1} & 27.9 & 04.8 & 17.5 & 41.5 & 42.9 & \textbf{51.7} & 31.3 & 23.3 \\
   T\'ouche-2020 & \textbf{60.5} & 23.1 & 25.2 & 12.7 & 28.4 & 24.9 & 22.6 & \underline{37.8} & 27.5 & 39.9 & 38.2\\
   CQADupStack   & 31.6 & 25.7 & 23.6 & 15.3 & 29.6 & 30.6 & 33.9 & \underline{34.8} & \textbf{35.0} \\
   Quora         & 74.2 & 63.0 & 76.7 & 24.8 & 85.2 & \textbf{85.5} & 85.3 & 77.8 & \underline{85.4} & 74.2 & 84.9 \\
   DBPedia       & 28.8 & 31.4 & 23.8 & 26.3 & 28.1 & 33.9 & 32.0 & \underline{38.0} & \textbf{39.2} & 21.8 & \colorbox{green!30}{35.8} \\
   SCIDOCS       & \textbf{15.6} & 12.6 & 10.4 & 07.7 & 12.2 & 13.3 & 14.8 & \underline{15.4} & 14.5 & 14.8 & 15.4 \\
   FEVER         & 64.8 & 59.6 & 54.6 & 56.2 & 66.9 & 67.0 & 64.1 & \textbf{79.3} & \underline{77.1} & 61.8 & \colorbox{green!30}{74.5} \\
   Climate-FEVER & 17.9 & 08.2 & 11.3 & 14.8 & 19.8 & 20.5 & \underline{22.0} & \textbf{24.6} & 18.4 & 14.0 & 19.6 \\
   SciFact       & \underline{62.0} & 58.2 & 31.2 & 31.8 & 50.7 & 53.1 & 59.2 & 52.4 & \textbf{67.1} & 67.5 & {69.1} \\ \midrule
   AVERAGE       & 41.9 & 34.6 & 28.0 & 23.3 & 39.1 & 38.8 & 40.1 & \textbf{44.7} & \underline{43.7} \\
        \bottomrule
    \end{tabular}}
    \caption{In-domain and Zero-shot retrieval performances on \beir datasets. All scores denote \textbf{nDCG@10}. The best retrieval performance on a given dataset is marked in \textbf{bold}, and the second best performance is \underline{underlined}. Corresponding Recall@100 performances can be found in \autoref{tab:results-recall}. $\ddagger$ indicates the in-domain performances. In-domain and zero-shot retrieval performance on \beir datasets. Scores denote \textbf{Recall@100}. The best retrieval performance on a given dataset is marked in \textbf{bold}, and the second best performance is \underline{underlined}. $\ddagger$ indicates in-domain retrieval performance. $^\star$ indicates the capped recall score: R\_cap@100 (\autoref{sec:capped_recall_score}). }
    \label{tab:results}
\end{table*}

%%%%%%%%%%%%%%%%%%%%%%%%%%%%%%%%%%%%%%%%%%%%%%%%%%%%%%%%%

\begin{table*}[t!]
    \tiny
    \resizebox{\textwidth}{!}{\begin{tabular}{l | c | c | c c c c c | c c | c c }
        \toprule
        \multicolumn{1}{l}{\textbf{Model ($\rightarrow$)}} &
        \multicolumn{1}{c}{Lexical}   &
        \multicolumn{1}{c}{Sparse}   &
        \multicolumn{5}{c}{Dense / Neural} &
        \multicolumn{2}{c}{Reranking} &
        \multicolumn{2}{c}{Our retrievers} \\ 
        \cmidrule(lr){1-1}
        \cmidrule(lr){2-2}
        \cmidrule(lr){3-3}
        \cmidrule(lr){4-8}
        \cmidrule(lr){9-10}
        \cmidrule(lr){11-12}
        \multicolumn{1}{l}{\textbf{Dataset ($\downarrow$)}} &
        \multicolumn{1}{c}{\textbf{BM25}} &
        \multicolumn{1}{c}{\textbf{SPARTA}} &
        \multicolumn{1}{c}{\textbf{USE-QA}} &
        \multicolumn{1}{c}{\textbf{DPR}} &
        \multicolumn{1}{c}{\textbf{ANCE}} &
        \multicolumn{1}{c}{\textbf{SBERT}} &
        \multicolumn{1}{c}{\textbf{GenQ}} &
        \multicolumn{1}{c}{\textbf{BM25+CE}} &
        \multicolumn{1}{c}{\textbf{ColBERT}} &
        \multicolumn{1}{c}{\textbf{Zero-shot}} &
        \multicolumn{1}{c}{\textbf{After finetuning}} \\
        \midrule

   MSMARCO & 0.218 & 0.351$^\ddagger$ & 0.259 & 0.177 & 0.388$^\ddagger$ & \underline{0.389}$^\ddagger$ & \underline{0.389}$^\ddagger$ & 0.384$^\ddagger$ & \textbf{0.425}$^\ddagger$ & 0.168 & 0.356\\  \midrule \midrule
   TREC-COVID    & 0.616 & 0.538 & 0.528 & 0.332 & 0.654 & 0.482 & 0.554 & \underline{0.667} & \textbf{0.677} & 0.214 & 0.438 \\
   BioASQ        & \textbf{0.514} & 0.351 & 0.093 & 0.127 & 0.306 & 0.295 & 0.351 & \underline{0.489} & 0.474 \\
   NFCorpus      & 0.297 & 0.301 & 0.252 & 0.189 & 0.237 & 0.257 & 0.293 & \underline{0.303} & \textbf{0.305} &  0.299 & \colorbox{blue!30}{0.324}\\ \midrule
   NQ            & 0.310 & 0.398 & 0.180 & 0.474$^\ddagger$ & 0.446 & 0.450 & 0.360 & \underline{0.516} & \textbf{0.524} &  0.184 & 0.443 \\ 
   HotpotQA      & \underline{0.601} & 0.492 & 0.258 & 0.391 & 0.456 & 0.513 & 0.497 & \textbf{0.701} & 0.593 & 0.384 & \colorbox{green!30}{0.644} \\ 
   FiQA-2018     & 0.239 & 0.198 & 0.264 & 0.112 & 0.295 & 0.258 & 0.284 & \textbf{0.326} & \underline{0.317} & 0.168 & 0.277\\ \midrule
   Signal-1M (RT)& \textbf{0.388} & 0.252 & 0.241 & 0.155 & 0.249 & 0.261 & 0.257 & \underline{0.308} & 0.274 \\ \midrule
   TREC-NEWS     & 0.371 & 0.258 & 0.340 & 0.161 & 0.382 & 0.367 & 0.369 & \textbf{0.430} & \underline{0.393} \\ \midrule
   ArguAna       & \underline{0.441} & 0.279 & 0.048 & 0.175 & 0.415 & 0.429 & \textbf{0.517} & 0.313 & 0.233 \\  
   T\'ouche-2020 & \textbf{0.605} & 0.231 & 0.252 & 0.127 & 0.284 & 0.249 & 0.226 & \underline{0.378} & 0.275 & 0.399 & 0.382\\ \midrule 
   CQADupStack   & 0.316 & 0.257 & 0.236 & 0.153 & 0.296 & 0.306 & 0.339 & \underline{0.348} & \textbf{0.350} \\
   Quora         & 0.742 & 0.630 & 0.767 & 0.248 & 0.852 & \textbf{0.855} & 0.853 & 0.778 & \underline{0.854} & 0.742 & 0.849 \\ \midrule
   DBPedia       & 0.288 & 0.314 & 0.238 & 0.263 & 0.281 & 0.339 & 0.320 & \underline{0.380} & \textbf{0.392} & 0.218 & \colorbox{green!30}{0.358} \\ \midrule
   SCIDOCS       & \textbf{0.156} & 0.126 & 0.104 & 0.077 & 0.122 & 0.133 & 0.148 & \underline{0.154} & 0.145 & 0.148 & 0.154 \\ \midrule
   FEVER         & 0.648 & 0.596 & 0.546 & 0.562 & 0.669 & 0.670 & 0.641 & \textbf{0.793} & \underline{0.771} & 0.618 & \colorbox{green!30}{0.745} \\ 
   Climate-FEVER & 0.179 & 0.082 & 0.113 & 0.148 & 0.198 & 0.205 & \underline{0.220} & \textbf{0.246} & 0.184 & 0.140 & 0.196 \\ 
   SciFact       & \underline{0.620} & 0.582 & 0.312 & 0.318 & 0.507 & 0.531 & 0.592 & 0.524 & \textbf{0.671} & 0.675 & \colorbox{blue!30}{0.691} \\ \midrule
   AVERAGE       & 0.419 & 0.346 & 0.280 & 0.233 & 0.391 & 0.388 & 0.401 & \textbf{0.447} & \underline{0.437} \\ 
        \bottomrule
    \end{tabular}}
    \caption{In-domain and Zero-shot retrieval performances on \beir datasets. All scores denote \textbf{nDCG@10}. The best retrieval performance on a given dataset is marked in \textbf{bold}, and the second best performance is \underline{underlined}. Corresponding Recall@100 performances can be found in \autoref{tab:results-recall}. $\ddagger$ indicates the in-domain performances.}
    \label{tab:results}
\end{table*}

\begin{table*}[t!]
    \tiny
    \resizebox{\textwidth}{!}{\begin{tabular}{l | c | c | c c c c c | c c | c c}
        \toprule
        \multicolumn{1}{l}{\textbf{Model ($\rightarrow$)}} &
        \multicolumn{1}{c}{Lexical}   &
        \multicolumn{1}{c}{Sparse}   &
        \multicolumn{5}{c}{Dense / Neural} &
        \multicolumn{2}{c}{Reranking} &
        \multicolumn{2}{c}{My retrievers} \\ 
        \cmidrule(lr){1-1}
        \cmidrule(lr){2-2}
        \cmidrule(lr){3-3}
        \cmidrule(lr){4-8}
        \cmidrule(lr){9-10}
        \cmidrule(lr){11-12}
        \multicolumn{1}{l}{\textbf{Dataset ($\downarrow$)}} &
        \multicolumn{1}{c}{\textbf{BM25}} &
        \multicolumn{1}{c}{\textbf{SPARTA}} &
        \multicolumn{1}{c}{\textbf{USE-QA}} &
        \multicolumn{1}{c}{\textbf{DPR}} &
        \multicolumn{1}{c}{\textbf{ANCE}} &
        \multicolumn{1}{c}{\textbf{SBERT}} &
        \multicolumn{1}{c}{\textbf{GenQ}} &
        \multicolumn{1}{c}{\textbf{BM25+CE}} &
        \multicolumn{1}{c}{\textbf{ColBERT}} & 
        \multicolumn{1}{c}{\textbf{Zero-shot}} &
        \multicolumn{1}{c}{\textbf{After finetuning}}\\
        \midrule
%  Dataset       & BM25  & SPARTA&  USE  & DPR   & ANCE  &MSMARCO& GenQ  & Rerank&ColBERT\\ 
   MSMARCO       & 0.621 & 0.793$^\ddagger$ & 0.720 & 0.552 & \underline{0.852}$^\ddagger$ & 0.847$^\ddagger$ & 0.847$^\ddagger$ & 0.621$^\ddagger$ &  \textbf{0.865}$^\ddagger$ & 0.609 & \colorbox{blue!30}{0.875} \\ \midrule
   TREC-COVID    & 0.447$^\star$ & 0.409$^\star$ & 0.339$^\star$ & 0.212$^\star$ & \underline{0.457}$^\star$ & 0.344$^\star$ & 0.442$^\star$ & 0.447$^\star$ & \textbf{0.464}$^\star$ \\
   BioASQ        & \textbf{0.716} & 0.351 & 0.145 & 0.256 & 0.463 & 0.466 & 0.577 & \textbf{0.716} & \underline{0.645} \\
   NFCorpus      & 0.196 & 0.243 & \textbf{0.273} & 0.208 & 0.232 & 0.235 & \underline{0.272} & 0.196 & 0.254 & \colorbox{blue!30}{0.285} & \colorbox{blue!30}{0.292} \\ \midrule
   NQ            & 0.753 & 0.787 & 0.605 & \underline{0.880}$^\ddagger$ & 0.836 & 0.858 & 0.845 & 0.753 & \textbf{0.912} & 0.672 & \colorbox{blue!30}{0.918} \\ 
   HotpotQA      & \textbf{0.757} & 0.651 & 0.398 & 0.591 & 0.578 & 0.637 & 0.624 & \textbf{0.757} & \underline{0.748} & 0.610 & \colorbox{blue!30}{0.791}\\ 
   FiQA-2018     & 0.505 & 0.446 & 0.601 & 0.342 & 0.581 & 0.540 & \textbf{0.609} & 0.505 & \underline{0.603} & 0.440 & 0.595\\ \midrule
   Signal-1M (RT)& \textbf{0.376} & 0.270 & 0.266 & 0.162 & 0.239 & 0.263 & 0.271 & \textbf{0.376} & \underline{0.283} \\ \midrule
   TREC-NEWS     & \textbf{0.401} & 0.262 & 0.381 & 0.215 & \underline{0.398} & 0.367 & 0.395 & \textbf{0.401} & 0.367 \\ \midrule
   ArguAna       & 0.931 & 0.893 & 0.454 & 0.751 & 0.937 & \underline{0.945} & \textbf{0.979} & 0.931 & 0.914 & 0.928 & 0.927 \\  
   T\'ouche-2020 & \textbf{0.463} & 0.257 & 0.257 & 0.171 & 0.307 & 0.300 & 0.273 & \textbf{0.463} & \underline{0.309} & 0.263 & 0.250 \\ \midrule 
   CQADupStack   & 0.588 & 0.521 & 0.546 & 0.403 & 0.579 & 0.596 & \textbf{0.672} & 0.588 & \underline{0.624} \\
   Quora         & 0.948 & 0.896 & 0.978 & 0.470 & \underline{0.987} & \textbf{0.989} & \textbf{0.989} & 0.948 & \textbf{0.989} & 0.959 & \colorbox{blue!30}{0.989} \\ \midrule
   DBPedia       & 0.384 & \underline{0.411} & 0.281 & 0.349 & 0.319 & 0.403 & 0.396 & 0.384 & \textbf{0.461} & 0.379 & \colorbox{blue!30}{0.515} \\ \midrule
   SCIDOCS       & \textbf{0.346} & 0.297 & 0.255 & 0.219 & 0.269 & 0.296 & 0.334 & \textbf{0.346} & \underline{0.344} & \colorbox{blue!30}{0.368} & \colorbox{blue!30}{0.362}\\ \midrule
   FEVER         & 0.908 & 0.843 & 0.850 & 0.840 & 0.900 & 0.914 & \underline{0.920} & 0.908 & \textbf{0.934} & 0.920 & \colorbox{blue!30}{0.947} \\ 
   Climate-FEVER & 0.383 & 0.227 & 0.346 & 0.390 & 0.445 & \underline{0.448} & \textbf{0.517} & 0.383 & 0.444 & 0.463 & 0.492 \\ 
   SciFact       & 0.838 & 0.863 & 0.631 & 0.727 & 0.816 & 0.849 & \textbf{0.892} & 0.838 & \underline{0.878} & \colorbox{blue!30}{0.961} & \colorbox{blue!30}{0.936} \\ \midrule
   AVERAGE       & 0.587 & 0.523 & 0.463  & 0.430 & 0.566 & 0.572 & \underline{0.603} & 0.587 & \textbf{0.613} \\ 
        \bottomrule
    \end{tabular}}
    \caption{In-domain and zero-shot retrieval performance on \beir datasets. Scores denote \textbf{Recall@100}. The best retrieval performance on a given dataset is marked in \textbf{bold}, and the second best performance is \underline{underlined}. $\ddagger$ indicates in-domain retrieval performance. $^\star$ indicates the capped recall score: R\_cap@100 (\autoref{sec:capped_recall_score}). }
    \label{tab:results-recall}
\end{table*}

\subsection{Open Domain Question Answering}

The standard approach for question answering consists in \emph{retriever-reader} approach.
Given an input question, the \emph{retriever}, selects relevant documents in a knowledge source. Then the \emph{reader} takes as input these retrieved passages along with the question in order to generate an answer.
We consider two settings to show that our pretrained model improves performance over Bert from which we start our contrastive pretraining.
In this section we show that initializing the retriever with our pretrained model instead of the pretrained model with masked language modeling improve the retriever performance after finetuning in two different settings. 
Interestingly, on NaturalQuestions and TriviaQA, after finetuning on MSMarco our retriever exhibits stronger retrieval performance than DPR which has been specifically trained on these datasets as well as competitive zero-shot performance with BM25.

\subsubsection{DPR}

\begin{table}[h!]
\centering
\begin{tabular}{l|cccc | cccc} 
 \toprule
  & \multicolumn{4}{c}{NaturalQuestions} & \multicolumn{4}{c}{TriviaQA} \\
  & R@5 & R@20 & R@100 & EM & R@5 & R@20 & R@100 & EM\\ 
 \midrule
 DPR~\citep{karpukhin2020dense} & - &  78.4 & 85.4 & & - & 79.4 & 85.0\\ 
 Our DPR & 67.6 & 79.4 & 86.0 & & & & &\\
 With pretrained model & 69.3 & 81.6 & 87.7 & 48.0 & 74.0 & 81.5 & 86.4\\
 With pretrained model - hard neg setting & 73.0 & 83.0 & 88.5 & 48.1 \\
 \bottomrule
\end{tabular}
\caption{Performance on the test set of NaturalQuestions and TriviaQA in the setting of DPR~\citep{karpukhin2020dense}.}
\label{tab:dpr}
\end{table}

\begin{table}[h!]
\centering
\begin{tabular}{l|cccc|cccc} 
 \toprule
  & \multicolumn{4}{c}{NaturalQuestions} & \multicolumn{4}{c}{TriviaQA} \\
  & R@5 & R@20 & R@100 & EM &  R@5 & R@20 & R@100 & EM\\ 
 \midrule
 DPR~\citep{karpukhin2020dense} & - &  78.4 & 85.4 & & - & 79.4 & 85.0\\ 
 BM25 (probably need better baselines) & - & 59.1 & 73.7 & & - & 66.9 & 76.7\\
 
 Zero-shot & 40.8 & 61.2 & 76.7 & & 53.9 &  69.9 & 80.8 & 60.3\\
 After MSMarco finetuning & 62.2 & 78.1 & 86.7 & \\
 After MSMarco finetuning, 4nodes, asam rho=2 & 64.4 & 79.0 & 87.4 & 48.2 & 71.3 & 80.0 & 85.7 & 67.2\\
 \bottomrule
\end{tabular}
\caption{Performance on the test set of NaturalQuestions and TriviaQA in the setting of DPR~\citep{karpukhin2020dense}.}
\label{tab:qa_zs}
\end{table}

\subsubsection{Distilling knowledge from reader to retriever}

\begin{table}[h!]
\centering
\begin{tabular}{l|cccc|cccc} 
 \toprule
  & \multicolumn{4}{c}{NaturalQuestions} & \multicolumn{4}{c}{TriviaQA} \\
  & R@5 & R@20 & R@100 & EM &  R@5 & R@20 & R@100 & EM \\ 
 \midrule
 First iteration \citep{izacard2021distilling} & - & 80.3 & 86.7 & 47.8 & - & 81.4 & 86.4 & 67.1 \\
 Second iteration \citep{izacard2021distilling} & - & 82.4 & 87.9 & 48.2 & - & 83.5 & 87.4 & 68.1 \\
 With pretrained 1st iter dpr documents & 70.3 & 81.2 & 87.4 & 48.5 \\
 With pretrained 2nd iter dpr documents & 73.0 & 83.1 & 88.1 & 49.3 \\
 With pretrained 1st iter dpr documents & 71.8 & 81.7 & 87.6 & 48.7 \\
 With pretrained 1st iter zeroshot documents & 69.4 & 80.1 & 86.3 & 48.0 & 74.6 & 82.4 & 86.6 & 68.2 \\
 With pretrained 2nd iter zeroshot documents & 71.9 & 82.9 & 88.0 & 49.1 & 75.7 & 83.3 & 87.0 & 68.6 \\
 With pretrained 1st iter msmarco documents & 72.6 & 82.6 & 87.9 & 49.5 & 76.9 & 83.6 & 87.6 & 68.9 \\ 
 With pretrained 2nd iter msmarco documents & 73.3 & 83.1 & 88.4 & 49.6 & 77.7 & 84.3 & 87.7 \\
 With pretrained 1st iter msmarco documents msmod & 73.0 & 83.0 & 88.2 & 49.2 \\ 
 \bottomrule
\end{tabular}
\caption{Performance on the dev set of NaturalQuestions and TriviaQA.}
\label{tab:qa_zs}
\end{table}

\begin{table}[h!]
\centering
\begin{tabular}{l|cccccc} 
 \toprule
  & \#training samples & Bert + contrastive & Bert & Bert + MSMarco &  wBert comparison & woBert \\
 \midrule
 Scifact & 809 & 86.1 & 77.6 & 82.0 & 80.4 & 78.8  \\
 NfCorpus & 2590 & 34.9 & 24.9 & 33.1 & 34.6 & 33.9 \\
 FiQA & 5500 & 31.5 & 26.5 & 30.5 & 30.1 & 22.9 \\
 HotpotQA & 85000 & 69.5 & 52.8 & 57.1 \\
 Fever & 109810 & 69.6 &  & 52.8 \\
 \bottomrule
\end{tabular}
\caption{Performance on the test sets after training on the train set of different datasets with different initialization.}
\label{tab:qa_zs}
\end{table}

\begin{table}[h!]
\centering
\begin{tabular}{l|cccccccccc} 
 \toprule
 & \multicolumn{2}{c}{WoW
} & \multicolumn{2}{c}{Hotpot} & \multicolumn{2}{c}{NQ} & \multicolumn{2}{c}{Fever} & \multicolumn{2}{c}{Eli5}  \\
& R-prec & R@5 & R-prec & R@5 & R-prec & R@5 & R-prec & R@5 & R-prec & R@5\\ \midrule
Wiki pretraining + msmarco & 32.1 & 57.5 & 44.3 & 31.8 & 48.9 & 66.3 & 68.8 & 87.8 & 13.3 & 25.6 \\
Multi-DPR & 41.0 & 67.1 & 42.9 & 28.4 & 59.4 & 68.2 & 74.5 & 87.5 & 15.5 & 27.5 \\
 \bottomrule
\end{tabular}
\caption{KILT}
\label{tab:kilt}
\end{table}

\begin{table}[h!]
\centering
\begin{tabular}{l|cccccccccccc} 
 \toprule
 & \multicolumn{2}{c}{FeverMin
} & \multicolumn{2}{c}{ClimateFeverMin} & \multicolumn{2}{c}{Nfcorpus} & \multicolumn{2}{c}{NQ50k} & \multicolumn{2}{c}{Scidocs} & \multicolumn{2}{c}{Scifact}  \\
& ZS & AT & ZS & AT & ZS & AT & ZS & AT & ZS & AT & ZS & AT \\ \midrule
100k & & 92.4 & & 36.6 & & \\
200k & & 92.8 & & 36.3 & & \\
300k & & 93.2 & & 38.9 & & \\
400k & & 93.3 & & 38.6 & & \\
500k & & 93.2 & & 37.5 & & \\
 \bottomrule
\end{tabular}
\caption{Improvement with pretraining}
\label{tab:improvement}
\end{table}
